# Supplementary material for: An efficient Lagrangian-based heuristic to solve a multi-objective sustainable supply chain problem
Source: arXiv:1906.06375 source file (2021-01-07)
Supplement: Supplementary file 1 [file supplementary_Tautenhain2019_SSCM_Lagrangian_EJOR_v5.pdf]

# Supplementary material to the paper "An efficient Lagrangian-based heuristic to solve a multi-objective sustainable supply chain problem"

## 1 Adapted *AugMathFix*

This appendix shows the matheuristic *AugMathFix* originally introduced in [Tautenhain et al., 2018], and which we adapted in this paper to solve the model introduced in [Mota et al., 2018]. The pseudocode of the adapted method is presented in Algorithm 1.

First, let us present the problem with  $\epsilon$ -Constraints to be solved by the adapted *AugMathFix* – referred to as MOP in the paper.

$$(\text{MOP}) : \min \quad f_{eco}(u, v, w', w'') - \epsilon ps\left(\frac{l_{env}}{r_{env}} + 0.1 \frac{l_{soc}}{r_{soc}}\right) \quad (1)$$

$$s.t. \quad \mathcal{A}'u + \mathcal{A}''v \leq \beta' + \beta''w'' \quad (2)$$

$$E'u + E''v \leq d \quad (3)$$

$$f_{env}(u, v, w', w'') + l_{env} = \epsilon_{env} \quad (4)$$

$$f_{soc}(u, v, w', w'') + l_{soc} = \epsilon_{soc} \quad (5)$$

$$u \in \mathbb{R}_{\geq 0}, v \in \mathbb{Z}_{\geq 0}^n, w' \in \{0, 1\}^{b'}, w'' \in \{0, 1\}^{b''} \quad (6)$$

$$l_{env}, l_{soc} \in \mathbb{R}_{\geq 0} \quad (7)$$

The adapted *AugMathFix* is an iterative AUGMECON2-based matheuristic that solves a sequence of mono-objective problems MOP by a heuristic method known as *MathFix*. These problems are generated by varying the values of  $\epsilon$  as in *AugMathLagr*. Therefore, the pseudocode of *AugMathFix* – Algorithm 1 – is the same as *AugMathLagr* except for line 10, which corresponds to the solution method to solve the MOP.

*MathFix* is a heuristic to solve mono-objective problems based on the fixing and re-solving strategy. Algorithm 2 shows a pseudocode of this heuristic.

The inputs of Algorithm 2 are the original MOP, referred to as  $P^{(0)}$ , the maximum number of iterations of the algorithm,  $IT$ , and positive real scalars  $\alpha, \beta, \theta, dec\alpha, dec\beta$  and  $dec\theta$  such that  $\alpha + \beta + \theta = 1$  and  $dec\alpha + dec\beta + dec\theta = 0$ . More details about these scalars can be found in the paper that first proposed the method. The values employed are the ones suggested in [Tautenhain et al., 2018]. Therefore, the following parameter values were employed in the experiments described in this paper:  $IT = 5, \alpha = 0.5, \beta = 0.5, \theta = 0, dec\alpha = -0.25, dec\beta = 0$  and  $dec\theta = -0.25$ .

In the first line of Algorithm 2, a relax-and-fix heuristic in *MathFix*, called *Heuristic*, is used to solve the initial problem  $P^{(0)}$ . The pseudocode of the *Heuristic* is presented in Algorithm 3 and shall be discussed later. Alike the original *Mathfix*, a control variable  $ch$  dictates the choice for defining the closing of entities. In this adaptation, we consider two alternatives: if the choice is 0, i.e., if value 0 is assigned to  $ch$  the option is to close a warehouse; if  $ch$  is 1, the option is to close a factory. Moreover,

---

**Algorithm 1:** Adapted *AugMathFix*.

---

**Input** : maximum number of iterations,  $kMax$ , step size  $st$ , number of grid points  $dg$

**Output:** Pareto frontier approximation  $\mathcal{P}$

```
1 Estimate the lower bounds  $fL_i$  and the upper bounds  $fU_i$ ,  $i \in \{eco, env, soc\}$  for the objective
  functions
2 Identify ranges  $r_j = fU_j - fL_j$ ,  $j \in \{env, soc\}$  of the environmental and social objective functions,
  respectively
3  $step_j = \frac{r_j}{d_j}$ ,  $j \in \{env, soc\}$ 
4  $\mathcal{P} := \emptyset$ 
5  $gr_{env} = 0$ 
6 for  $\epsilon_{env} = fU_{env}$  until  $gr_{env} < dg$  do
7    $gr_{soc} = 0$ 
8   for  $\epsilon_{soc} = fU_{soc}$  until  $gr_{soc} < dg$  do
9      $MOP := \text{Problem (1)-(7)}$ 
10     $x_f := \text{solve MOP using Algorithm 2 - MathFix - considering } \epsilon_{env} \text{ and } \epsilon_{soc}$ 
11    if  $x_f$  is feasible then
12       $\mathcal{P} := \mathcal{P} \cup x_f$ 
13       $gr_{soc} = gr_{soc} + 1 + \lfloor \frac{l_{soc}}{step_{soc}} \rfloor$ 
14       $\epsilon_{soc} = \epsilon_{soc} - step_{soc} \left( 1 + \lfloor \frac{l_{soc}}{step_{soc}} \rfloor \right)$ 
15    else  $gr_{soc} = dg$  ;
16  end
17   $gr_{env} = gr_{env} + 1$ 
18   $\epsilon_{env} = \epsilon_{env} - step_{env}$ 
19 end
20  $\mathcal{P} := \text{Remove dominated solutions from } \mathcal{P}$ 
21 return  $\mathcal{P}$ 
```

---

in line 2, auxiliary variables of the algorithm related to this choice are initialized:  $num_o = 0$  (number of times that choice  $o$  was applied in the heuristic) and  $max_o = IT$  (maximum number of times that choice  $o$  can be applied in the heuristic before restarting the problem), for each option  $o \in \{0, 1\}$ .

At each iteration of *MathFix*,  $veco_i$ ,  $venv_i$  and  $vuse_i$  are defined in lines 6, 7 and 8 as, respectively, the economic cost, the environmental impact and the storage or production related to warehouse or factory  $i$ . In line 7,  $wwh$ ,  $wpt$  and  $wpsq_i$  are, respectively, the number of weekly working hours, the number of weeks per time period and the minimum number of workers per square meter in entity  $i \in I_f \cup I_w$ . In line 9, if  $ch = 1$ ,  $\mathcal{I}$  is defined as the warehouse  $i$  whose sum  $\alpha veco_i + \beta venv_i + \theta vuse_i$  is the minimum amongst all  $i \in I_w$ . If  $ch = 0$ , in line 10,  $\mathcal{I}$  is defined as the factory  $i$  whose value of  $\alpha veco_i + \beta venv_i + \theta vuse_i$  is the minimum amongst all  $i \in I_f$ . In line 11,  $P^{(it)}$  is obtained by fixing  $Y_i = 0$ ,  $YC_i = 0$ ,  $KT_{ait} = 0$ ,  $K_{ai} = 0$  and  $S_{mit} = 0$  and removing the constraints  $S_{mit} \geq ic_{mi}^{min} Y_i$ ,  $m \in M_{fp}$ ,  $a \in A$ ,  $t \in T$  and  $YC_i \geq ea_i^{min} Y_i$  at  $P^{(it-1)}$ . Moreover, if  $ch = 1$ , i.e.,  $i$  is a factory,  $P_{mgit} = 0$ ,  $(m, g) \in H_{prod}$ , and  $R_{mgit} = 0$ ,  $(m, i) \in H_{rem}$  and the constraints  $P_{mgit} \geq pc_g^{min} Z_{gmi}$ ,  $(m, g) \in H_{prod}$  and  $R_{mgit} \geq pc_g^{min} Z_{gmi}$ ,  $(m, g) \in H_{rem}$ ,  $t \in T$  are also removed. In line 12, *Heuristic* is applied to  $P^{(it)}$  and its solution is called  $x_{FS}^{(it)}$ . If solution  $x_{FS}^{(it)}$  is feasible,  $num_{ch}$  is incremented in line 14. The best solution achieved up to the current iteration  $x^{best}$  is checked for update in line 15. In lines 16 and 17,  $ch$  is updated to either 1 or 0, depending on its current value. In case  $num_{ch} \geq max_{ch}$ , the problem and feasible solution of the current iteration are reset to the respective problem and feasible solution of the first iteration. Moreover,  $max_{ch}$  is limited by  $num_{ch}$ . In case  $x_{FS}^{(it)}$  is infeasible,  $\alpha$ ,  $\beta$  and  $\theta$  are updated in line 23. At the end, Algorithm 2 returns the best solution found over the iterations,  $x^{best}$ .

Algorithm 3 presents the heuristic to solve an input problem  $P^{(it)}$ .

In line 1 of Algorithm 3, the linear relaxation of problem  $P^{(it)}$  is assigned to  $PR^{(it)}$ . In line 2, the

---

**Algorithm 2:** *MathFix*.

---

**Input :** Problem  $P^{(0)}$ , maximum number of iterations,  $IT$  and positive scalars  $\alpha, \beta, \theta, dec\alpha, dec\beta$  and  $dec\theta$  such that  $\alpha + \beta + \theta = 1$  and  $dec\alpha + dec\beta + dec\theta = 0$

**Output:** The best feasible solution  $x^{best}$

```
1  $x_{FS}^{(0)} := Heuristic(P^{(0)})$ 
2  $num_o = 0, max_o = IT, o \in \{0, 1\}$ 
3  $x^{best} := x_{FS}^{(0)}$ 
4  $it = 1, ch = 0$ 
5 while  $it < IT$  do
6    $vuse_i = \sum_{t \in T} \sum_{m \in M_{fp} \cup M_{rp}} S_{mit}, \forall i \in I_f \cup I_w$ 
7    $veco_i = sqmc_i YC_i + lc_i wwh wpt wpsq_i YC_i + lc_i w_i wwh wpt, \forall i \in I_f \cup I_w$ 
8    $venv_i = \arg \min_{i \in I_w} \sum_{c \in C} (\eta_c e_{ic} YC_i), \forall i \in I_f \cup I_w$ 
9   if  $ch = 0$  then  $\mathcal{I} := \arg \min_{i \in I_w} (\alpha vuse_i + \beta veco_i + \theta venv_i)$  ;
10  else if  $ch = 1$  then  $\mathcal{I} := \arg \min_{i \in I_f} (\alpha vuse_i + \beta veco_i + \theta venv_i)$  ;
11   $P^{(it)} :=$  Fix non-binary variables index by  $\mathcal{I}$  at problem  $P^{(it-1)}$ 
12   $x_{FS}^{(it)} := Heuristic(P^{(it)})$ 
13  if  $x_{FS}^{(it)}$  is feasible then
14     $num_{ch} = num_{ch} + 1$ 
15    if  $f_{eco}(x_{FS}^{(it)}) > f_{eco}(x^{best})$  then  $x^{best} := x_{FS}^{(it)}$  ;
16    if  $ch = 0$  then  $ch = 1$ ;
17    else if  $ch = 1$  then  $ch = 0$ ;
18    if  $num_{ch} \geq max_{ch}$  then
19       $P^{(it)} := P^{(0)}, x_{FS}^{(it)} := x_{FS}^{(0)}$ 
20       $max_{ch} = num_{ch}, num_o = 0, o \in \{0, 1\}$ 
21    end
22  else
23     $\alpha = \alpha + dec\alpha, \beta = \beta + dec\beta, \theta = \theta + dec\theta$ 
24  end
25   $it = it + 1$ 
26 end
27 return  $x^{best}$ 
```

---

problem is solved using the CPLEX solver. Then, the problem given as input is assigned to  $P_{FS}^{(it)}$  and in the next lines of the algorithm some variables of  $P_{FS}^{(it)}$  are fixed according to the values of the variables of the solution of the linear relaxation. Accordingly, the variables  $Y_i$ , for all the values of  $i$  that meet the conditions in lines 4 to 7, are fixed at 1 in problem  $PR_{RS}^{it}$ . Variables  $Y_i$  and  $Z_{gmi}$  that are not fixed at 0 are fixed at 1 in lines 8 and 9.

Consider the transportation constraints given by Equations (8) - (10). Constraints (8) calculate the number of trucks of each type required by each entity in each time period; Constraints (9) define the upper bound on the number of trucks required over the entire planning horizon; Constraint (10) establishes a maximum investment of  $invt$  (€) in trucks.

$$KT_{ait} = \frac{\sum_j 2d_{ij} Q_{aijt}}{avs.mhw.wpt}, \quad a \in A_{truck}, i \in I, t \in T \quad (8)$$

$$K_{ai} \geq KT_{ait}, \quad a \in A_{truck}, i \in I, t \in T \quad (9)$$

$$\sum_{a \in A_{truck}, i \in I} ftc_a K_{ai} \leq invt \quad (10)$$

From lines 12 to 23, the values of the variables  $Q_{aijt}$ ,  $a \in A_{truck}, i, j \in I, t \in T$  are inspected to set lower bounds to the related variables  $K_{ait}$  and  $K_{ai}$  that satisfy Constraint (10). In line 17,  $Q_{aijt}^{(it)}$  is the value of  $Q_{aijt}$  in  $x_{RL}^{(it)}$ .

---

**Algorithm 3: Heuristic.**

---

**Input** : Problem  $P^{(it)}$   
**Output**: Feasible solution  $x_{FS}^{(it)}$

```
1  $PR_{RL}^{(it)} :=$  Linear relaxation of problem  $P^{(it)}$ 
2  $x_{RL}^{(it)} :=$  Solve  $PR_{RL}^{(it)}$ 
3  $P_{FS}^{(it)} := P^{(it)}$ 
4 forall  $i, j$  such that  $\sum_{t \in T} \sum_{m \in M_{rm}, a \in A} X_{mai jt} > 0$  in  $x_{RL}^{(it)}$  do Fix  $Y_i = 1$  and  $Y_j = 1$  at problem  $P_{FS}^{(it)}$  ;
5 forall  $i \in I_w$  such that  $S_{mit} > 0, m \in M_{fp}, t \in T$ , in  $x_{RL}^{(it)}$  do Fix  $Y_i = 1$  at problem  $P_{FS}^{(it)}$  ;
6 forall  $i \in I_f, (m, g) \in H_{prod}, t \in T$  such that  $P_{mgit} > 0$ , in  $x_{RL}^{(it)}$  do Fix  $Y_i = 1$  and  $Z_{gmi} = 1$  at problem  $P_{FS}^{(it)}$  ;
7 forall  $i \in I_f, (m, g) \in H_{rem}, t \in T$  such that  $R_{mgit} > 0$  in  $x_{RL}^{(it)}$  do Fix  $Y_i = 1$  and  $Z_{gmi} = 1$  at problem  $P_{FS}^{(it)}$  ;
8 if  $Y_i$  is not fixed at 1 then Fix  $Y_i = 0$  at problem  $P_{FS}^{(it)}$ ;
9 if  $Z_{gmi}$  is not fixed at 1 then Fix  $Z_{gmi} = 0$  at problem  $P_{FS}^{(it)}$ ;
10  $acc = 0$ 
11 for  $a \in A_{truck}, i \in I$  do
12   for  $t \in T$  do
13      $sum = 0$ 
14     for  $j \in I$  do
15        $sum = sum + \frac{2d_{ij}Q_{aijt}}{avs.mhw.wpt}$ 
16       if  $(acc + \lceil sum \rceil) \leq invt$  then
17         Add the following constraint to problem  $P_{FS}^{(it)}$ :  $Q_{aijt} \geq Q_{aijt}^{(it)}$ 
18     end
19     Add the following constraint to problem  $P_{FS}^{(it)}$ :  $K_{ait} \geq sum$ 
20   end
21    $max =$  maximum lower bound of  $K_{ait}$  over  $t \in T$ 
22    $acc = acc + max$ 
23   Add the following constraint to problem  $P_{FS}^{(it)}$ :  $K_{ai} \geq max$ 
24 end
25  $x_{FS}^{(it)} :=$  Solve  $P_{FS}^{(it)}$ 
26 return  $x_{FS}^{(it)}$ 
```

---

A feasible solution  $x_{FS}^{(it)}$  is obtained by solving problem  $P_{FS}^{(it)}$  using CPLEX in line 25 and is returned in line 26.

## 2 Generator parameters values

This section presents the values of the generator used in the experiments reported here.

- $lbdc = 8336.8, ubdc = 34481.28$ , and  $vart = 0.1$ ;
- $lbBOM^{prod} = 0.015, ubBOM^{prod} = 0.45, lbBOM^{rem} = 4$  and  $ubBOM^{rem} = 5$ ;
- $lbpu = 0.1$  and  $ubpu = 0.9$ ;
- $lbapu = 0.001$  and  $ubapu = 0.004$ ;
- $wbret = 0.15$  and  $fracwg = 10$ ;
- $icfrac^{max} = 0.5$  and  $icfrac^{min} = 0.01$ ;
- $lbpc^{min} = 0.0005$ ;

- $lbeaf^{max} = 10000, ubeaf^{max} = 12500, lbeaw^{max} = 4000$  and  $ubeaw^{max} = 4750$ ;
- $lbeaf^{min} = 100, ubeaf^{min} = 1000, lbeaw^{min} = 25$  and  $ubeaw^{min} = 250$ ;
- $lpsc = 0.00001$  and  $upsc = 0.0001$ ;
- $lbtec = 0.025$  and  $ubtech = 0.037$ ;
- $lbopc = 0.150$  and  $ubopc = 0.4$ .
- $lbpsu = 23$  and  $ubpsu = 37$ ;
- $scfrac = 0.01$ ;
- $lbrpc = 0.005$  and  $ubrpc = 0.5$ ;
- $lbrmc = 0.01$  and  $ubrmc = 0.27$ ;
- $lbsqmc = 0.5, ubsqmc = 50$  and  $sqmcfac = 1.25$ ;
- $lbwf = 5, ubwf = 6, lbww = 4$  and  $ubww = 5$ ;
- $lbpsqf = 0.01, ubpsqf = 0.01, lbwpsqw = 0.03$  and  $ubwpsqw = 0.03$ .

Moreover, the remaining parameters of the model studied by Mota et al. [2018] and their fixed values are given by:

- fuel price  $fp = 1.7$  (€/per  $l$ );
- vehicle maintenance costs  $vmc = 0.3$  (€);
- average vehicle speed  $avs = 60$  ( $km/h$ );
- maximum driving hours per week  $mhw = 45$ ;
- number of weeks per time period  $wpt = 17.33$ ;
- number of weekly working hours  $wwh = 40$ ;
- average vehicle consumption  $avc_a \in [14, 18], a \in A_{truck}$  ( $l$  per  $100km$ );
- number of workers in the transportation  $w_a = 1, a \in A_{truck}$  ;
- Maximum investment in trucks  $invt = 2000000$  (€);
- interest rate  $ir = 0.1$ ;
- salvage value  $sv = 0.2$ ;
- tax rate  $tx = 0.3$ .

### 3 Illustrative example data

Tables 1 to 7 show the data regarding the illustrative example presented in Section 5.4 of the paper.

Table 1 presents the parameters of each item. We refer to raw materials as  $rm_0$  and  $rm_1$ , to the final product as  $fp_0$  and to the recovered product as  $rp_0$ . The lifetime of the final product is one period.

Table 1: Illustrative example: data related to items.

| Data                    | $rm_0$ | $rm_1$ | $fp_0$    | $rp_0$    |
|-------------------------|--------|--------|-----------|-----------|
| Return rate             | -      | -      | -         | 0.0549277 |
| Recovery cost (€)       | -      | -      | -         | 9.55536   |
| Stock cost (€)          | -      | -      | 0.0149574 | 0         |
| Selling price (€)       | -      | -      | 34.995    | -         |
| Product weight ( $kg$ ) | 0.127  | 0.185  | 0.050     | 0.249     |
| Required area ( $m^2$ ) | 0.001  | 0.002  | 0.001     | 0.003     |

Table 2 reports the production and remanufacturing technologies. We refer to technologies as  $G = G_{prod} \cup G_{rem}$ , where  $G_{prod} = \{g_0, g_1, g_2\}$  and  $G_{rem} = \{g_3, g_4, g_5\}$ .

Table 2: Illustrative example: technology specifications.

| Data                         | $g_0$ | $g_1$ | $g_2$ | $g_3$ | $g_4$ | $g_5$ |
|------------------------------|-------|-------|-------|-------|-------|-------|
| Maximum capacity             | 44676 | 45679 | 39978 | 38236 | 44339 | 46553 |
| Minimum capacity             | 0     | 0     | 0     | 0     | 0     | 0     |
| Installation Cost (€)        | 1247  | 1329  | 1439  | 1028  | 1146  | 1322  |
| Operation costs per unit (€) | 0.354 | 0.303 | 0.376 | 0.187 | 0.400 | 0.396 |

Table 3 defines the bill of raw materials required by a production technology to produce final products.

Table 3: Illustrative example: bill of raw materials for production.

|        | $fp_0$ |       |       |
|--------|--------|-------|-------|
|        | $g_0$  | $g_1$ | $g_2$ |
| $rm_0$ | 0.123  | 0.381 | 0.105 |
| $rm_1$ | 0.391  | 0.113 | 0.165 |

The amount of recovered products  $rp_0$  required by any remanufacturing technology to obtain the final product  $fp_0$  is 5.

Table 4 presents the maximum capacity, the minimum order and the unit cost of the raw materials for each supplier.

Table 4: Illustrative example: supplier related data.

| Data                      | $rm_0$   | $rm_1$    |
|---------------------------|----------|-----------|
| Maximum supplier capacity | 108928   | 96840     |
| Minimum order             | 5        | 4         |
| Raw material cost (€)     | 0.156347 | 0.0258353 |

Table 5 presents the parameters related to the installation and operation of the factories and warehouses.

Table 5: Illustrative example: installation and operation of the factory and warehouses.

| Data                                     | Factory | Warehouse 1 | Warehouse 2 |
|------------------------------------------|---------|-------------|-------------|
| Maximum installation area ( $m^2$ )      | 2272    | 892         | 836         |
| Minimum installation area ( $m^2$ )      | 54      | 30          | 43          |
| Construction cost (€)                    | 6228    | 5836        | 5841        |
| Fixed number of workers                  | 1       | 1           | 0           |
| Fixed number of workers per square meter | 0.002   | 0.001       | 0.002       |
| Maximum storage                          | -       | 39146       | 36893       |
| Minimum storage level                    | -       | 391         | 368         |

Table 6 details the labour cost and GDP index of each entity.

Table 6: Illustrative example: labour cost and GDP index of each entity.

| Entity      | Labour cost | GDP index |
|-------------|-------------|-----------|
| Supplier    | 30.245      | 0.572     |
| Factory     | 10.958      | 0.74      |
| Warehouse 1 | 21.299      | 0.861     |
| Warehouse 2 | 27.92       | 0.421     |
| Customer 1  | 27.277      | 1.188     |
| Customer 2  | 5.933       | 0.773     |
| Airport 1   | 13.639      | 0.915     |
| Airport 2   | 28.207      | 0.956     |
| Seaport 1   | 7.663       | 1.226     |
| Seaport 2   | 18.628      | 0.803     |

Table 7 describes the transportation specifications for each mode, which we refer to as  $K = \{k_0, k_1, k_2, k_3\}$ .

Table 7: Illustrative example: data related to transportation.

| Data                                    | $k_0$    | $k_1$    | $k_2$   | $k_3$   |
|-----------------------------------------|----------|----------|---------|---------|
| Maximum transportation capacity         | 52377    | 54504    | 400000  | 500000  |
| Minimum transportation                  | 0        | 0        | 0       | 0       |
| Maximum contracted units                | -        | -        | 3000000 | 3000000 |
| Fixed transportation cost (€)           | 96627    | 87103    | 4000000 | 4000000 |
| Fixed number of workers                 | 1        | 1        | 0       | 0       |
| Vehicle consumption ( $l$ per $100km$ ) | 18       | 15       | -       | -       |
| Maximum investment on trucks (€)        | 13716710 | 13716710 | -       | -       |

The investments, as well as their salvage values and depreciation rates; and the fixed parameter values are defined according to the case study presented in [Mota et al., 2018]. They are shown in Section 4 of this supplementary material.

Table 8 details the demand of the customers for final products in each period of the planning horizon.

Table 8: Illustrative example: demand for final products.

| Final Product | Customer   | Planning period $t \in T$ |       |       |
|---------------|------------|---------------------------|-------|-------|
|               |            | 1                         | 2     | 3     |
| $fp_0$        | Customer 1 | 14895                     | 16384 | 18023 |
|               | Customer 2 | 12528                     | 13781 | 15159 |

Tables 9, 10 and 11 show the environmental impacts of installing entities by using, respectively, production and remanufacturing technologies and transportation modes.

Table 9: Illustrative example: environmental impact on entity installation, per  $m^2$  of entity area.

| Impact category | Environmental impact per $m^2$ of entity area. |
|-----------------|------------------------------------------------|
| CC              | 82612.041                                      |
| OD              | 21939.939                                      |
| TA              | 24797.047                                      |
| FE              | 81280.902                                      |
| ME              | 46016.221                                      |
| HT              | 76412.059                                      |
| POF             | 63497.697                                      |
| PMF             | 49721.387                                      |
| TET             | 37345.676                                      |
| FET             | 64471.149                                      |
| MET             | 65295.073                                      |
| IR              | 52890.036                                      |
| ALO             | 66265.249                                      |
| ULO             | 39267.008                                      |
| NLT             | 69005.33                                       |
| MRD             | 8356.2                                         |
| FRD             | 5347.654                                       |

Table 10: Illustrative example: environmental impact resulting from the use of technology per kilogram of product produced or remanufactured.

| Impact category | Environmental impact per $kg$ produced or remanufactured. |            |            |            |            |            |
|-----------------|-----------------------------------------------------------|------------|------------|------------|------------|------------|
|                 | $g_0$                                                     | $g_1$      | $g_2$      | $g_3$      | $g_4$      | $g_5$      |
| CC              | 210120.507                                                | 230767.701 | 74750.833  | 27157.828  | 93404.67   | 379750.088 |
| OD              | 301007.767                                                | 435759.524 | 200319.033 | 350671.788 | 401081.367 | 117987.282 |
| TA              | 247888.673                                                | 430041.032 | 448535.44  | 127199.718 | 218901.199 | 330934.938 |
| FE              | 440598.94                                                 | 138700.425 | 109190.333 | 360359.71  | 70537.035  | 68253.735  |
| ME              | 19388.193                                                 | 288075.111 | 225731.139 | 181922.07  | 414621.059 | 442205.277 |
| HT              | 1075.716                                                  | 243544.61  | 33124.89   | 394432.162 | 220422.137 | 397460.129 |
| POF             | 64068.708                                                 | 434766.741 | 239947.812 | 99142.95   | 427939.753 | 374738.739 |
| PMF             | 67938.75                                                  | 297073.265 | 115906.014 | 21040.483  | 157449.8   | 198709.26  |
| TET             | 91691.729                                                 | 251985.538 | 277920.455 | 44441.083  | 193805.298 | 450702.193 |
| FET             | 86369.791                                                 | 289347.153 | 357246.65  | 375536.064 | 67408.427  | 152868.785 |
| MET             | 48082.5                                                   | 91851.341  | 386452.911 | 107381.762 | 53418.982  | 274171.031 |
| IR              | 159791.308                                                | 148911.536 | 284027.889 | 355751.987 | 99959.859  | 8312.942   |
| ALO             | 408108.968                                                | 409499.795 | 11510.356  | 174853.967 | 86683.948  | 2608.231   |
| ULO             | 74783.198                                                 | 118635.371 | 195645.937 | 392006.597 | 196628.775 | 154100.17  |
| NLT             | 300396.11                                                 | 452523.988 | 429418.414 | 350896.322 | 129851.12  | 106293.507 |
| MRD             | 100833.497                                                | 19961.464  | 170858.402 | 447148.05  | 348070.812 | 59490.558  |
| FRD             | 302240.943                                                | 17385.897  | 5063.264   | 7082.493   | 177477.589 | 322209.56  |

Table 11: Illustrative example: environmental impact resulting from the transportation per  $kg$  of item and per  $km$ .

| Impact category | Environmental impact per $kg$ and $km$ transported |       |       |       |
|-----------------|----------------------------------------------------|-------|-------|-------|
|                 | $k_0$                                              | $k_1$ | $k_2$ | $k_3$ |
| CC              | 0.002                                              | 0.003 | 0.001 | 0.002 |
| OD              | 0.001                                              | 0.001 | 0.002 | 0.002 |
| TA              | 0                                                  | 0.002 | 0.002 | 0.003 |
| FE              | 0                                                  | 0.002 | 0.003 | 0.002 |
| ME              | 0                                                  | 0.001 | 0.002 | 0.001 |
| HT              | 0.003                                              | 0.001 | 0     | 0.002 |
| POF             | 0.001                                              | 0.001 | 0.001 | 0.001 |
| PMF             | 0.001                                              | 0.002 | 0     | 0.001 |
| TET             | 0.003                                              | 0.002 | 0.003 | 0.001 |
| FET             | 0                                                  | 0.003 | 0.001 | 0.002 |
| MET             | 0.002                                              | 0.001 | 0.002 | 0.001 |
| IR              | 0                                                  | 0.002 | 0.003 | 0.001 |
| ALO             | 0.002                                              | 0.003 | 0.001 | 0.002 |
| ULO             | 0.001                                              | 0.002 | 0.002 | 0.003 |
| NLT             | 0.001                                              | 0     | 0.002 | 0.001 |
| MRD             | 0.002                                              | 0.003 | 0.002 | 0.002 |
| FRD             | 0.001                                              | 0.001 | 0.001 | 0     |

Table 24 presents the normalization factors for each impact category.

## 4 Case study from [Mota et al., 2018]

This section presents the data employed the case study from [Mota et al., 2018].

Table 12 presents the parameters of each item. We refer to raw materials as  $rm_0, rm_1, rm_2$  and  $rm_3$ , to final products as  $fp_0$  and  $fp_1$  and to recovered products as  $rp_0$  and  $rp_1$ .

Table 12: Case study: parameters of each item.

|                                              | Raw material |        |        |        | Final product |        | Recovered product |        |
|----------------------------------------------|--------------|--------|--------|--------|---------------|--------|-------------------|--------|
|                                              | $rm_0$       | $rm_1$ | $rm_2$ | $rm_3$ | $fp_0$        | $fp_1$ | $rp_0$            | $rp_1$ |
| Product recovery cost (€)                    | -            | -      | -      | -      | -             | -      | 0.15              | 0.15   |
| Inventory cost per unit (€)                  | -            | -      | -      | -      | 0.01          | 0.01   | -                 | -      |
| Price per unit sold (€)                      | -            | -      | -      | -      | 23            | 37     | -                 | -      |
| Product weight ( $kg$ )                      | 0.118        | 0.184  | 0.365  | 0.913  | 0.4           | 0.5    | 0.4               | 0.5    |
| Necessary area per unit of product ( $m^2$ ) | 0.002        | 0.001  | 0.004  | 0.003  | 0.007         | 0.009  | 0.007             | 0.009  |

Table 13 specifies the production and remanufacturing technologies. The production technologies are  $gp1, gp1alt, gp2$  and  $gp2alt$ , whereas the remanufacturing technologies are  $gr1$  and  $gr2$ .

Table 13: Case study: technology specifications.

| Technology                   | Production |          |         |          | Remanufacturing |         |
|------------------------------|------------|----------|---------|----------|-----------------|---------|
|                              | $gp1$      | $gp1alt$ | $gp2$   | $gp2alt$ | $gr1$           | $gr2$   |
| Maximum capacity             | 5800000    | 6000000  | 4600000 | 5200000  | 2900000         | 2300000 |
| Minimum capacity             | 30000      | 30000    | 30000   | 30000    | 0               | 0       |
| Installation Cost (€)        | 150000     | 175000   | 167000  | 186000   | 50000           | 45000   |
| Operation costs per unit (€) | 0.212      | 0.196    | 0.324   | 0.267    | 0.116           | 0.134   |
| Number of workers            | 2          | 1        | 4       | 3        | 1               | 1       |

Table 14 defines the bill of raw materials required by a production technology to produce final products. Technologies  $gp1$  and  $gp1al$  can produce  $fp_0$  and  $gp2$  and  $gp2alt$  can produce  $fp_1$ .

Table 14: Case study: bill of raw materials for production.

|        | $fp_0$ |         | $fp_1$ |          |
|--------|--------|---------|--------|----------|
|        | $gp1$  | $gp1al$ | $gp2$  | $gp2alt$ |
| $rm_0$ | 0.25   | 0.25    | 0.45   | 0.42     |
| $rm_1$ | 0.3    | 0.3     | 0.4    | 0.2      |
| $rm_2$ | 0.15   | 0.05    | 0.025  | 0.015    |
| $rm_3$ | 0.3    | 0.2     | 0.42   | 0.3      |

Table 15 defines the amount of recovered products required by a remanufacturing technology to obtain a final product.

Table 15: Case study: remanufacturing bill.

|        | $fp_0$ | $fp_1$ |
|--------|--------|--------|
|        | $gr1$  | $gr2$  |
| $rp_0$ | 4      | 0      |
| $rp_1$ | 0      | 5      |

Table 16 presents the maximum capacity, the minimum order and the unit cost of the raw materials for each supplier.

Table 16: Case study: raw material parameters for each supplier.

|                  | Supplier | Raw material |         |         |         |
|------------------|----------|--------------|---------|---------|---------|
|                  |          | $rm_0$       | $rm_1$  | $rm_2$  | $rm_3$  |
| Maximum capacity | Verona   | 3600000      | 3600000 | 1000000 | 4000000 |
|                  | Hannover | 3800000      | 3800000 | 1200000 | 5000000 |
|                  | Leeds    | 3800000      | 3800000 | 1200000 | 5000000 |
| Minimum order    | Verona   | 1000         | 1000    | 200     | 1000    |
|                  | Hannover | 0            | 0       | 0       | 0       |
|                  | Leeds    | 0            | 0       | 0       | 0       |
| Unit cost (€)    | Verona   | 0.01         | 0.025   | 0.03    | 0.09    |
|                  | Hannover | 0.035        | 0.0875  | 0.105   | 0.315   |
|                  | Leeds    | 0.03         | 0.075   | 0.09    | 0.27    |

The factory and the warehouse in Verona are already installed with capacities of 20000  $m^2$  and 5000  $m^2$ , respectively. Table 17 presents the parameters related to the installation and operation of the remaining factories and warehouses.

Table 17: Case study: installation and operation of the factory and warehouses.

| Data                                     | Factories | Warehouses |
|------------------------------------------|-----------|------------|
| Maximum installation area ( $m^2$ )      | 25000     | 8000       |
| Minimum installation area ( $m^2$ )      | 2000      | 500        |
| Fixed number of workers                  | 11        | 9          |
| Fixed number of workers per square meter | 0.01      | 0.01       |
| Maximum storage                          | -         | 1200000    |
| Minimum storage level                    | -         | 391        |

Only warehouses stock products in this case study. The maximum storage capacity for final products  $fp_0$  and  $fp_1$  are, respectively, 1200000 and 1000000. The minimum inventory levels for  $fp_0$  and  $fp_1$  are, respectively, 12000 and 10000 units.

Table 18 describes the transportation specifications for each mode, that is, land ( $A_{truck}$ ), air ( $A_{plane}$ ) and sea ( $A_{boat}$ ). The land transportation mode uses trucks  $Truck1$  and  $Truck2$ ; the air transportation mode uses airplanes  $Air1$ ,  $Air2$ ,  $Air3$  and  $Air4$ ; and the sea transportation uses boats  $Boat1$  and  $Boat2$ . In this table, (\*) indicates that the transportation cost per kilogram in truck  $a \in A_{truck}$  is calculated according to Equation (11).

Table 18: Case study: transportation specifications.

|                                              | Land     |          | Air     |        |        |        | Sea     |         |
|----------------------------------------------|----------|----------|---------|--------|--------|--------|---------|---------|
|                                              | $Truck1$ | $Truck2$ | $Air1$  | $Air2$ | $Air3$ | $Air4$ | $Boat1$ | $Boat2$ |
| Maximum capacity                             | 35,000   | 55,000   | 400,000 |        |        |        | 500,000 |         |
| Minimum units transported                    | 200      | 200      | 1000    |        |        |        | 1,000   |         |
| Maximum contracted capacity per time period  | -        | -        | 3000000 |        |        |        | 3000000 |         |
| Fixed costs (€)                              | 30000    | 50000    | 108000  | 126000 | 126000 | 72000  | 144000  | 72000   |
| Handling costs at hub terminals per unit(€)  | -        | -        | 0.100   | 0.125  | 0.125  | 0.075  | 0.150   | 0.075   |
| Transportation cost per kg (€)               | *        | *        | 0.04    |        |        |        | 0.01    |         |
| Necessary workers per unit                   | 1        | 1        | 0       |        |        |        | 0       |         |
| Average vehicle consumption ( $L/per100km$ ) | 14       | 18       | -       | -      | -      | -      | -       | -       |

$$tc_a = \frac{avc_a}{100}fp + vmc \quad (11)$$

There are three types of investments: investments in entities, technologies and transportation. Their savage values are, respectively, 0.5, 0 and 0. The depreciation rates of the investments at each time period are presented in Table 19.

Table 19: Case study: depreciation rates of entities.

| Investment     | Planning period $t \in T$ |       |       |       |       |       |       |       |      |      |
|----------------|---------------------------|-------|-------|-------|-------|-------|-------|-------|------|------|
|                | 1                         | 2     | 3     | 4     | 5     | 6     | 7     | 8     | 9    | 10   |
| Entities       | 0.05                      | 0.05  | 0.05  | 0.05  | 0.05  | 0.05  | 0.05  | 0.05  | 0.05 | 0.05 |
| Technologies   | 0.125                     | 0.125 | 0.125 | 0.125 | 0.125 | 0.125 | 0.125 | 0.125 | 0    | 0    |
| Transportation | 0.2                       | 0.2   | 0.2   | 0.2   | 0.2   | 0     | 0     | 0     | 0    | 0    |

Table 20 details the demand of the customers for final products in each period of the planning horizon.

Table 20: Case study: demand for final products.

| Final Product | Customer  | Planning period $t \in T$ |         |         |         |         |         |         |         |         |         |
|---------------|-----------|---------------------------|---------|---------|---------|---------|---------|---------|---------|---------|---------|
|               |           | 1                         | 2       | 3       | 4       | 5       | 6       | 7       | 8       | 9       | 10      |
| $fp_1$        | Verona    | 2873448                   | 2077056 | 2527512 | 2761104 | 2873448 | 2077056 | 2527512 | 2761104 | 2873448 | 2077056 |
|               | Hannover  | 1789152                   | 2125200 | 1963824 | 1731192 | 1789152 | 2125200 | 1963824 | 1731192 | 1789152 | 2125200 |
|               | Leeds     | 1138848                   | 1940424 | 1693848 | 1730232 | 1138848 | 1940424 | 1693848 | 1730232 | 1138848 | 1940424 |
|               | Zaragoza  | 1221432                   | 1706760 | 1416312 | 1413504 | 1221432 | 1706760 | 1416312 | 1413504 | 1221432 | 1706760 |
|               | Lisbon    | 1128840                   | 1147512 | 1180632 | 1291368 | 1128840 | 1147512 | 1180632 | 1291368 | 1128840 | 1147512 |
|               | São Paulo | 919464                    | 1414368 | 1014696 | 1146216 | 919464  | 1414368 | 1014696 | 1146216 | 919464  | 1414368 |
|               | Recife    | 1443216                   | 1513152 | 1676112 | 1217544 | 1443216 | 1513152 | 1676112 | 1217544 | 1443216 | 1513152 |
| $fp_2$        | Verona    | 1518120                   | 2017416 | 1502280 | 2114616 | 1518120 | 2017416 | 1502280 | 2114616 | 1518120 | 2017416 |
|               | Hannover  | 1570152                   | 1836480 | 1396152 | 1962480 | 1570152 | 1836480 | 1396152 | 1962480 | 1570152 | 1836480 |
|               | Leeds     | 1033632                   | 1229904 | 1259544 | 1554048 | 1033632 | 1229904 | 1259544 | 1554048 | 1033632 | 1229904 |
|               | Zaragoza  | 825308                    | 706380  | 785482  | 769706  | 825308  | 706380  | 785482  | 769706  | 825308  | 706380  |
|               | Lisboa    | 1065288                   | 1055544 | 936192  | 1100112 | 1065288 | 1055544 | 936192  | 1100112 | 1065288 | 1055544 |
|               | São Paulo | 1390704                   | 1251432 | 991992  | 1570176 | 1390704 | 1251432 | 991992  | 1570176 | 1390704 | 1251432 |
|               | Recife    | 833688                    | 1362000 | 1547280 | 1426056 | 833688  | 1362000 | 1547280 | 1426056 | 833688  | 1362000 |

The analysis of the environmental impact assessed by ReCiPe2008 takes into account all the impact categories, i.e. Climate Change (CC), Ozone Depletion (OD), Terrestrial Acidification (TA), Freshwater Eutrophication (FE), Marine Eutrophication (ME), Human Toxicity (HT), Photochemical Oxidant Formation (POF), Particulate Matter Formation (PMF), Terrestrial Ecotoxicity (TE), Freshwater Ecotoxicity (FE), Marine Ecotoxicity (MET), Ionising Radiation (IR), Agricultural Land Occupation (ALO), Urban Land Occupation (ULO), Natural Land Transformation (NLT), Metal Depletion (MRD) and Fossil Depletion (FD).

Tables 21, 22 and 23 show the environmental impacts of installing entities that use production and remanufacturing technologies and transportation modes, respectively. Table 24 defines the normalization factors for each impact category.

Table 21: Case study: environmental impact on entity installation, per  $m^2$  of entity area.

| Impact category | Environmental impact per $m^2$ of entity area. |
|-----------------|------------------------------------------------|
| CC              | 3.78E+02                                       |
| OD              | 2.23E-05                                       |
| TA              | 4.02E+00                                       |
| FE              | 1.24E-01                                       |
| ME              | 1.66E-01                                       |
| HT              | 8.32E+02                                       |
| POF             | 2.18E+00                                       |
| PMF             | 1.38E+00                                       |
| TET             | 4.66E-01                                       |
| FET             | 1.21E+00                                       |
| MET             | -1.84E+01                                      |
| IR              | 7.67E+00                                       |
| ALO             | 2.22E+02                                       |
| ULO             | 3.38E+00                                       |
| NLT             | 3.20E-02                                       |
| MRD             | 1.31E+02                                       |
| FRD             | 1.02E+02                                       |

Table 22: Case study: environmental impact on the technology use, per *kg* of unit produced or remanufactured.

| Impact category | Environmental impact per <i>kg</i> produced or remanufactured. |          |          |          |          |          |
|-----------------|----------------------------------------------------------------|----------|----------|----------|----------|----------|
|                 | gp1                                                            | gp1al    | gr1      | gp2      | gp2al    | gr2      |
| CC              | 5.36E+02                                                       | 3.75E+02 | 1.34E+02 | 5.14E+02 | 4.11E+02 | 1.03E+02 |
| OD              | 1.96E-05                                                       | 1.37E-05 | 4.90E-06 | 1.66E-05 | 1.33E-05 | 2.66E-06 |
| TA              | 4.93E+00                                                       | 3.45E+00 | 1.23E+00 | 3.96E+00 | 3.17E+00 | 6.33E-01 |
| FE              | 2.51E+00                                                       | 1.76E+00 | 6.28E-01 | 7.15E-01 | 5.72E-01 | 1.14E-01 |
| ME              | 3.43E-01                                                       | 2.40E-01 | 8.59E-02 | 1.72E-01 | 1.37E-01 | 2.74E-02 |
| HT              | 1.10E+03                                                       | 7.70E+02 | 2.75E+02 | 8.71E+02 | 6.97E+02 | 1.39E+02 |
| POF             | 3.23E+00                                                       | 2.26E+00 | 8.07E-01 | 1.96E+00 | 1.57E+00 | 3.14E-01 |
| PMF             | 1.85E+00                                                       | 1.30E+00 | 4.63E-01 | 1.57E+00 | 1.25E+00 | 2.51E-01 |
| TET             | 5.02E-01                                                       | 3.51E-01 | 1.26E-01 | 3.99E-01 | 3.19E-01 | 6.39E-02 |
| FET             | 8.51E+00                                                       | 5.96E+00 | 2.13E+00 | 1.36E+00 | 1.09E+00 | 2.18E-01 |
| MET             | 4.57E+03                                                       | 3.20E+03 | 1.14E+03 | 1.24E+03 | 9.95E+02 | 1.99E+02 |
| IR              | 1.14E+02                                                       | 7.95E+01 | 2.84E+01 | 1.36E+02 | 1.09E+02 | 2.17E+01 |
| ALO             | 1.49E+02                                                       | 1.04E+02 | 3.72E+01 | 1.45E+02 | 1.16E+02 | 2.32E+01 |
| ULO             | 1.65E+01                                                       | 1.16E+01 | 4.13E+00 | 1.06E+01 | 8.48E+00 | 1.70E+00 |
| NLT             | 1.15E-01                                                       | 8.05E-02 | 2.88E-02 | 7.57E-02 | 6.06E-02 | 1.21E-02 |
| MRD             | 7.17E+02                                                       | 5.02E+02 | 1.79E+02 | 1.47E+02 | 1.18E+02 | 2.35E+01 |
| FRD             | 1.38E+02                                                       | 9.64E+01 | 3.44E+01 | 1.24E+02 | 9.94E+01 | 1.99E+01 |

Table 23: Case study: environmental impact on transportation per *kg* and *km* transported.

| Impact category | Environmental impact per <i>kg</i> and <i>km</i> transported |          |           |          |
|-----------------|--------------------------------------------------------------|----------|-----------|----------|
|                 | truck1                                                       | truck2   | plane     | boat     |
| CC              | 1.80E-03                                                     | 4.34E-04 | 1.03E-03  | 1.09E-05 |
| OD              | 1.28E-10                                                     | 3.31E-11 | 7.70E-11  | 7.31E-13 |
| TA              | 8.29E-06                                                     | 1.26E-06 | 3.35E-06  | 2.34E-07 |
| FE              | 5.04E-07                                                     | 4.00E-08 | -1.07E-08 | 1.45E-09 |
| ME              | 4.43E-07                                                     | 7.07E-08 | 1.89E-07  | 6.13E-09 |
| HT              | 3.14E-03                                                     | 4.19E-04 | 6.54E-04  | 1.04E-05 |
| POF             | 1.25E-05                                                     | 2.18E-06 | 5.93E-06  | 1.73E-07 |
| PMF             | 3.87E-06                                                     | 7.02E-07 | 1.08E-06  | 6.89E-08 |
| TET             | 3.18E-06                                                     | 9.77E-07 | 3.01E-07  | 4.00E-09 |
| FET             | 5.80E-07                                                     | 1.81E-07 | 2.02E-07  | 2.13E-09 |
| MET             | 2.22E-03                                                     | 3.98E-04 | 3.56E-04  | 1.21E-05 |
| IR              | 1.61E-04                                                     | 2.53E-05 | 6.39E-05  | 1.25E-06 |
| ALO             | 3.68E-04                                                     | 1.09E-04 | 2.00E-04  | 1.27E-06 |
| ULO             | 7.43E-05                                                     | 2.85E-05 | 8.67E-06  | 1.03E-07 |
| NLT             | 5.12E-07                                                     | 1.39E-07 | 3.02E-07  | 2.87E-09 |
| MRD             | 3.71E-04                                                     | 5.25E-05 | 5.85E-06  | 4.89E-07 |
| FRD             | 6.64E-04                                                     | 1.68E-04 | 3.79E-04  | 3.74E-06 |

Table 24: Case study: normalization factors for environmental impact categories.

| Impact category | Normalization factor |
|-----------------|----------------------|
| CC              | 1.81E-04             |
| OD              | 2.66E+01             |
| TA              | 2.37E-02             |
| FE              | 3.45E+00             |
| ME              | 1.36E-01             |
| HT              | 6.89E-04             |
| POF             | 1.76E-02             |
| PMF             | 7.11E-02             |
| TET             | 1.23E-01             |
| FET             | 2.20E-01             |
| MET             | 1.48E-03             |
| IR              | 7.59E-04             |
| ALO             | 1.84E-04             |
| ULO             | 1.29E-03             |
| NLT             | 8.31E-02             |
| MRD             | 2.25E-03             |
| FRD             | 7.75E-04             |

## References

- B. Mota, M. I. Gomes, A. Carvalho, and A. P. Barbosa-Povoa. Sustainable supply chains: An integrated modeling approach under uncertainty. *Omega*, 77:32 – 57, 2018. ISSN 0305-0483.
- C. P. Tautenhain, A. P. Barbosa-Póvoa, and M. C. V. Nascimento. A multi-objective matheuristic for designing and planning sustainable supply chains. *Computers & Industrial Engineering*, 2018.
